# Supplementary material for: Image-Based Geolocation Using Large Vision-Language Models
Source: arXiv:2408.09474 source file (2024-08-18)
Supplement: Supplementary file 1 [file Appendix.tex]

\clearpage
\appendix

\section{Appendix}\label{sec:appendix}
